# Supplementary material for: PrIC3: Property Directed Reachability for MDPs
Source: arXiv:2004.14835 source file (2020-05-18)
Supplement: Supplementary file 1 [file table1_additional_results.tex]

\documentclass[paper=landscape,a4paper,parskip=half-,DIV=15,fontsize=11pt]{scrartcl}
\usepackage[utf8]{inputenc}
\usepackage[T1]{fontenc}
\usepackage{lmodern}
\usepackage{multirow}
\begin{document}
    \centering
    \small{}\begin{tabular}{ccrr||cccc|} 
  & $|S|$ & $Pr^{max}(s_I \models \diamond B)$ & $\lambda$ & w/o & lin & pol & hyb \\
    \multirow{3}{*}{BRP} & \multirow{3}{*}{1000} & \multirow{3}{*}{0.035} & 0.1 & / & / & / & / \\
      &   &   & 0.01 & 43/324/23.4 & 43/324/8.4 & / & MO \\
      &   &   & 0.005 & 27/188/13.4 & 27/188/3.1 & / & / \\
    \multirow{4}{*}{ZeroConf} & \multirow{4}{*}{10000} & \multirow{4}{*}{0.5} & 0.9 & / & / & 0/0/- & 0/0/- \\
      &   &   & 0.75 & / & / & 0/0/- & 0/0/- \\
      &   &   & 0.52 & / & / & 0/0/- & 0/0/- \\
      &   &   & 0.45 & 1/1/29.9 & 1/1/27.2 & 1/1/27.8 & 1/1/29.8 \\
    \multirow{4}{*}{ZeroConf} & \multirow{4}{*}{1000000000} & \multirow{4}{*}{~0.55} & 0.9 & / & / & 0/0/- & / \\
      &   &   & 0.75 & / & / & 0/0/- & / \\
      &   &   & 0.52 & / & / & / & / \\
      &   &   & 0.45 & 1/1/30.2 & 1/1/25.6 & 1/1/27.1 & 1/1/26.7 \\
    \multirow{4}{*}{Chain} & \multirow{4}{*}{1001} & \multirow{4}{*}{0.394} & 0.9 & 0/0/- & 0/0/- & 0/0/- & 0/0/- \\
      &   &   & 0.4 & 0/0/- & 0/0/- & 0/0/- & / \\
      &   &   & 0.35 & 1/431/83.0 & 1/431/60.3 & / & / \\
      &   &   & 0.3 & 1/357/80.9 & 1/357/54.8 & / & / \\
    \multirow{4}{*}{Chain} & \multirow{4}{*}{10001} & \multirow{4}{*}{0.394} & 0.9 & / & / & 0/0/- & 0/0/- \\
      &   &   & 0.48 & / & / & 0/0/- & / \\
      &   &   & 0.4 & / & / & 0/0/- & / \\
      &   &   & 0.3 & / & / & / & / \\
    \multirow{2}{*}{Chain} & \multirow{2}{*}{1000000000000} & \multirow{2}{*}{0.394} & 0.9 & / & / & 0/0/- & / \\
      &   &   & 0.4 & / & / & 0/0/- & / \\
    \multirow{4}{*}{DoubleChain} & \multirow{4}{*}{1002} & \multirow{4}{*}{0.215} & 0.9 & 0/0/- & 0/0/- & 0/0/- & 0/0/- \\
      &   &   & 0.3 & 0/0/- & / & 0/0/- & 0/0/- \\
      &   &   & 0.216 & 0/0/- & / & 0/0/- & / \\
      &   &   & 0.15 & / & / & / & / \\
    \multirow{3}{*}{DoubleChain} & \multirow{3}{*}{10002} & \multirow{3}{*}{0.22} & 0.9 & / & / & 0/0/- & 0/0/- \\
      &   &   & 0.3 & / & / & 0/0/- & 0/0/- \\
      &   &   & 0.24 & / & / & 0/0/- & / \\
    \multirow{2}{*}{DoubleChain} & \multirow{2}{*}{10000000} & \multirow{2}{*}{$2.6E^{-4}$} & 0.004 & / & / & TO & / \\
      &   &   & 0.00027 & / & / & 0/0/- & /
\end{tabular}\end{document}
